# Supplementary material for: Exact closed-form recurrence probabilities for biased random walks at any step number
Source: arXiv:2412.17994 ancillary file (2024-12-23)
Supplement: Supplementary file 1 [file SupplMat.pdf]

## Supplementary Material –
## Exact closed-form recurrence probabilities for biased random walks at any step number

Debendro Mookerjee and Sarah Kostinski[†]

## Obtaining Eq. 3 of the main text: Path enumeration approach to the survival probability

Let $R(N)$ be the probability that the walker remains in the positive half-line and never returns to the origin by the $N$th step. Thus the running sum of the sequence of unit steps, denoted as $\pm1$'s, must remain positive. We define $L(N)$ similarly, except that the walker remains in the negative half-line to the left of the origin (a negative running sum). The survival probability $S(N)$ is simply $S(N) = R(N) + L(N)$. Below we proceed to first obtain an expression for $R(N)$.

The probability that a particular sequence has $N_+$ steps to the right and $N_-$ steps to the left is $p^{N_+}q^{N_-}$. The total number of such sequences with $N = N_+ + N_-$ steps is $\binom{N}{N_-}$. Survival at the $N$th step requires that the random walker never returned to the origin up to step $N$, i.e. the running sum never reached 0. Therefore, only a fraction of the $\binom{N}{N_-}$ sequences should be considered. This fraction is

$$\frac{N_+ - N_-}{N} = \frac{N - 2N_-}{N} = 1 - \frac{2N_-}{N} \tag{S1}$$

and is given by the generalized ballot theorem or the cycle lemma.[1]

Because we require that $N_+ > N_-$ for the walker to remain in the positive half-line, it implies that $N_-$ is an integer in the range $0 \le N_- \le \lfloor \frac{N-1}{2} \rfloor$. We can thus enumerate the possible "good" paths remaining in the positive half-line and sum over their respective probabilities as

$$R(N) = \sum_{N_-=0}^{\lfloor \frac{N-1}{2} \rfloor} p^{N-N_-}q^{N_-}\left(1 - \frac{2N_-}{N}\right)\binom{N}{N_-} = p^N + \sum_{N_-=1}^{\lfloor \frac{N-1}{2} \rfloor} p^{N-N_-}q^{N_-}\left(1 - \frac{2N_-}{N}\right)\binom{N}{N_-}, \tag{S2}$$

where we have chosen the limits such that $N_+ > N_-$, or equivalently, $0 \le N_- \le \lfloor \frac{N-1}{2} \rfloor$.

Splitting Eq. S2 into two sums and using the binomial identities

$$\binom{N}{N_-} = \binom{N-1}{N_- - 1} + \binom{N-1}{N_-} \tag{S3}$$

and

$$\frac{2N_-}{N}\binom{N}{N_-} = 2\binom{N-1}{N_- - 1} \tag{S4}$$

for the first and second terms, respectively, yields

$$R(N) = p^N + \sum_{N_-=1}^{\lfloor \frac{N-1}{2} \rfloor} p^{N-N_-}q^{N_-}\left[\binom{N-1}{N_-} - \binom{N-1}{N_- - 1}\right]. \tag{S5}$$

Changing the limits of summation in the last term on the RHS,

$$\sum_{N_-=1}^{\lfloor \frac{N-1}{2} \rfloor} p^{N-N_-}q^{N_-}\binom{N-1}{N_- - 1} = \frac{q}{p}\sum_{N_-=0}^{\lfloor \frac{N-1}{2} \rfloor - 1} p^{N-N_-}q^{N_-}\binom{N-1}{N_-} \tag{S6}$$

and similarly for the other terms on the RHS of Eq. S5 gives

$$p^N + \sum_{N_-=1}^{\lfloor \frac{N-1}{2} \rfloor} p^{N-N_-}q^{N_-}\binom{N-1}{N_-} = \sum_{N_-=0}^{\lfloor \frac{N-1}{2} \rfloor} p^{N-N_-}q^{N_-}\binom{N-1}{N_-}. \tag{S7}$$

[†]Department of Physics, New York University, New York, USA

Combining these yields

$$R(N) = p^{N-\lfloor \frac{N-1}{2} \rfloor} q^{\lfloor \frac{N-1}{2} \rfloor} \binom{N-1}{\lfloor \frac{N-1}{2} \rfloor} + \sum_{N_-=0}^{\lfloor \frac{N-1}{2} \rfloor - 1} \left( p^{N-N_-} q^{N_-} - p^{N-N_- -1} q^{N_- +1} \right) \binom{N-1}{N_-}. \tag{S8}$$

A similar expression can be obtained for $L(N)$, except now $N_- > N_+$. The fraction of paths remaining to the left of the origin is

$$\frac{N_- - N_+}{N} = \frac{N - 2N_+}{N} = 1 - \frac{2N_+}{N}, \tag{S9}$$

resulting in

$$L(N) = \sum_{N_+=0}^{\lfloor \frac{N-1}{2} \rfloor} p^{N_+} q^{N-N_+} \left(1 - \frac{2N_+}{N}\right) \binom{N}{N_+} = q^N + \sum_{N_+=1}^{\lfloor \frac{N-1}{2} \rfloor} q^{N-N_+} p^{N_+} \left[ \binom{N-1}{N_+} - \binom{N-1}{N_+ - 1} \right]$$

$$= q^{N-\lfloor \frac{N-1}{2} \rfloor} p^{\lfloor \frac{N-1}{2} \rfloor} \binom{N-1}{\lfloor \frac{N-1}{2} \rfloor} + \sum_{N_+=0}^{\lfloor \frac{N-1}{2} \rfloor - 1} \left( q^{N-N_+} p^{N_+} - q^{N-N_+ -1} p^{N_+ +1} \right) \binom{N-1}{N_+}. \tag{S10}$$

Note that $L(N)$ is the same as Eq. S8, but with $p$ and $q$ swapped. When computing $R(N) + L(N)$, we can treat $N_\pm$ as the same index $x$. Thus the survival probability is

$$S(N) = \left( p^{\lceil \frac{N+1}{2} \rceil} q^{\lfloor \frac{N-1}{2} \rfloor} + p^{\lfloor \frac{N-1}{2} \rfloor} q^{\lceil \frac{N+1}{2} \rceil} \right) \binom{N-1}{\lfloor \frac{N-1}{2} \rfloor} + (p-q) \sum_{x=0}^{\lfloor \frac{N-1}{2} \rfloor - 1} \left( p^{N-x-1} q^x - p^x q^{N-x-1} \right) \binom{N-1}{x}. \tag{S11}$$

In terms of the bias $B \equiv p - q$ where $p + q = 1$, the survival probability can be expressed simply in terms of $B$ as:

$$S(N,B) = 2^{-N} \left[ (1+B)^{\lceil \frac{N+1}{2} \rceil} (1-B)^{\lfloor \frac{N-1}{2} \rfloor} + (1+B)^{\lfloor \frac{N-1}{2} \rfloor} (1-B)^{\lceil \frac{N+1}{2} \rceil} \right] \binom{N-1}{\lfloor \frac{N-1}{2} \rfloor}$$

$$+ 2^{-(N-1)} B \sum_{x=0}^{\lfloor \frac{N-1}{2} \rfloor - 1} \left[ (1+B)^{N-x-1} (1-B)^x - (1+B)^x (1-B)^{N-x-1} \right] \binom{N-1}{x}. \tag{S12}$$

## Obtaining the survival probability in closed-form for odd step numbers (Eq. 4a of main text)

Let us denote the summation term in Eq. S12 as $\tilde{S}(N)$. Our aim is to find a closed-form expression for this summation. We define $\beta = \frac{1-B}{1+B}$ and express $\tilde{S}(N)$ in terms of $\beta$ as

$$\tilde{S}(N) = B \frac{(1+B)^{N-1}}{2^{N-1}} \left[ \sum_{x=0}^{\lfloor \frac{N-1}{2} \rfloor - 1} \left( \frac{1-B}{1+B} \right)^x \binom{N-1}{x} - \sum_{x=0}^{\lfloor \frac{N-1}{2} \rfloor - 1} \left( \frac{1-B}{1+B} \right)^{N-1-x} \binom{N-1}{x} \right]$$

$$= \frac{B(1+B)^{N-1}}{2^{N-1}} \left[ \sum_{x=0}^{\lfloor \frac{N-1}{2} \rfloor - 1} \beta^x \binom{N-1}{x} - \sum_{x=0}^{\lfloor \frac{N-1}{2} \rfloor - 1} \beta^{N-1-x} \binom{N-1}{x} \right]. \tag{S13}$$

Now let $y = N - 1 - x$ in the second summation in Eq. S13:

$$\tilde{S}(N) = \frac{B(1+B)^{N-1}}{2^{N-1}} \left[ \sum_{x=0}^{\lfloor \frac{N-1}{2} \rfloor - 1} \beta^x \binom{N-1}{x} - \sum_{y=N-\lfloor \frac{N-1}{2} \rfloor}^{N-1} \beta^y \binom{N-1}{N-1-y} \right]$$

$$= \frac{B(1+B)^{N-1}}{2^{N-1}} \left[ \sum_{x=0}^{\lfloor \frac{N-1}{2} \rfloor - 1} \beta^x \binom{N-1}{x} - \sum_{y=N-\lfloor \frac{N-1}{2} \rfloor}^{N-1} \beta^y \binom{N-1}{y} \right] \tag{S14}$$

and using the binomial theorem to rewrite the first summation, we obtain

$$\tilde{S}(N) = \frac{B(1+B)^{N-1}}{2^{N-1}} \left[ (1+\beta)^{N-1} - \sum_{x=\lfloor \frac{N-1}{2} \rfloor}^{N-1} \beta^x \binom{N-1}{x} - \sum_{y=N-\lfloor \frac{N-1}{2} \rfloor}^{N-1} \beta^y \binom{N-1}{y} \right]. \tag{S15}$$

Since we first consider odd steps $N$ here, let $N = 2m + 1$. We can thus simplify the floor functions as follows:

$$\left\lfloor \frac{N-1}{2} \right\rfloor = \frac{N-1}{2} = m; \qquad N - \left\lfloor \frac{N-1}{2} \right\rfloor = N - \left(\frac{N-1}{2}\right) = \frac{N+1}{2} = m+1\,. \tag{S16}$$

Eq. S15 then becomes

$$\tilde{S} = \frac{B(1+B)^{N-1}}{2^{N-1}}\left[(1+\beta)^{N-1} - \sum_{x=m}^{2m}\beta^x\binom{2m}{x} - \sum_{y=m+1}^{2m}\beta^y\binom{2m}{y}\right] = \frac{B(1+B)^{N-1}}{2^{N-1}}\left[(1+\beta)^{N-1} - \beta^m\binom{2m}{m} - 2\sum_{y=m+1}^{2m}\beta^y\binom{2m}{y}\right]. \tag{S17}$$

Noting that $(m-1)! = (m-1)(m-2)\cdots(2m+1-y)(2m-y)!$, the remaining summation can be rewritten as:

$$\begin{aligned}\sum_{y=m+1}^{2m}\beta^y\binom{2m}{y} &= \sum_{y=m+1}^{2m}\beta^y\frac{(2m)!}{y!(2m-y)!} = \sum_{y=m+1}^{2m}\frac{(2m)!}{y!}\beta^y\frac{(m-1)(m-2)\cdots(2m+1-y)}{(m-1)!}\\ &= \sum_{y=m+1}^{2m}\frac{(2m+1-y)\cdots(m-2)(m-1)}{y(y-1)\cdots(m+3)(m+2)}\frac{\beta^{y-m-1}(2m)!\beta^{m+1}}{(m+1)!(m-1)!}\\ &= \frac{\beta^{m+1}(2m)!}{(m+1)!(m-1)!}\sum_{y=m+1}^{2m}\frac{(2m+1-y)...(m-2)(m-1)\beta^{y-m-1}}{y(y-1)...(m+3)(m+2)}\,.\end{aligned} \tag{S18}$$

Letting $n = y - m - 1$, Eq. S18 becomes

$$\sum_{y=m+1}^{2m}\beta^y\binom{2m}{y} = \frac{\beta^{m+1}(2m)!}{(m+1)!(m-1)!}\sum_{n=0}^{m-1}\frac{(m-n)(m-n+1)\cdots(m-2)(m-1)}{(m+n+1)(m+n)\cdots(m+3)(m+2)}\beta^n\,. \tag{S19}$$

We now multiply and divide the summand by $n!$, and then multiply the summand by $(-1)^{2n}$:

$$\sum_{y=m+1}^{2m}\beta^y\binom{2m}{y} = \frac{\beta^{m+1}(2m)!}{(m+1)!(m-1)!}\sum_{n=0}^{m-1}\frac{n!}{n!}\frac{(m-n)(m-n+1)...(m-2)(m-1)(-1)^{2n}}{(m+n+1)(m+n)...(m+3)(m+2)}\beta^n\,. \tag{S20}$$

Next we pair a factor $(-1)^n$ with $\beta^n$, and pair the other $(-1)^n$ factor with $(m-n)(m-n+1)...(m-2)(m-1)$ to give $(1-m)(2-m)...(1-m+n-1)$:

$$\sum_{y=m+1}^{2m}\beta^y\binom{2m}{y} = \frac{\beta^{m+1}(2m)!}{(m+1)!(m-1)!}\sum_{n=0}^{m-1}\frac{n!\,(m-n)(m-n+1)...(m-2)(m-1)(-1)^n}{(m+n+1)(m+n)...(m+3)(m+2)}\frac{(-\beta)^n}{n!} \tag{S21}$$

$$= \frac{\beta^{m+1}(2m)!}{(m+1)!(m-1)!}\sum_{n=0}^{m-1}\frac{\big[(1)(2)...(1+n-1)\big]\big[(1-m)(2-m)...(1-m+n-1)\big]}{(2+m)(3+m)...(m+n+1)}\frac{(-\beta)^n}{n!}\,. \tag{S22}$$

We use the the falling Pochhammer symbol[2] $(r)_n$, defined as:

$$(r)_n = \begin{cases}1 & n=0\\ r(r+1)\cdots(r+n-1) & n>0\end{cases}, \tag{S23}$$

to write the sum as

$$\sum_{y=m+1}^{2m}\beta^y\binom{2m}{y} = \frac{\beta^{m+1}(2m)!}{(m+1)!(m-1)!}\sum_{n=0}^{m-1}\frac{(1)_n(1-m)_n}{(m+2)_n}\frac{(-\beta)^n}{n!} \tag{S24}$$

Because $(1-m)_n = 0$ for all $n > m-1$, this finite sum can be written as an infinite sum whose terms with index $n > m-1$ are zero-valued, thereby leading to a Gauss hypergeometric function:

$$\sum_{y=m+1}^{2m}\beta^y\binom{2m}{y} = \frac{\beta^{m+1}(2m)!}{(m+1)!(m-1)!}\sum_{n=0}^{\infty}\frac{(1)_n(1-m)_n}{(m+2)_n}\frac{(-\beta)^n}{n!} = \frac{\beta^{m+1}(2m)!}{(m+1)!(m-1)!}\,{}_2F_1(1;1-m;m+2;-\beta)\,. \tag{S25}$$

Combining this result with Eqs. S12 and S17 yields the following expression for the survival probability for odd $N$:

$$S_{\text{odd}} =\left[\frac{(1+B)^{\frac{N+1}{2}}(1-B)^{\frac{N-1}{2}}+(1+B)^{\frac{N-1}{2}}(1-B)^{\frac{N+1}{2}}}{2^N}\right]\binom{N-1}{\frac{N-1}{2}}+\frac{B(1+B)^{N-1}}{2^{N-1}}\left[\left(\frac{2}{1+B}\right)^{N-1}-\left(\frac{1-B}{1+B}\right)^{\frac{N-1}{2}}\binom{N-1}{\frac{N-1}{2}}\right.$$
$$\left.-\frac{2(N-1)!}{(\frac{N+1}{2})!(\frac{N-3}{2})!}\left(\frac{1-B}{1+B}\right)^{\frac{N+1}{2}}{}_2F_1\left(1;1-\frac{N-1}{2};\frac{N+3}{2};\frac{B-1}{B+1}\right)\right] \tag{S26}$$

The first term of Eq. S26 can be simplified as follows:

$$\left[\frac{(1+B)^{\frac{N+1}{2}}(1-B)^{\frac{N-1}{2}}+(1+B)^{\frac{N-1}{2}}(1-B)^{\frac{N+1}{2}}}{2^N}\right]\binom{N-1}{\frac{N-1}{2}}=\frac{(1-B^2)^{\frac{N}{2}}}{2^N}\left[\sqrt{\frac{1+B}{1-B}}+\sqrt{\frac{1-B}{1+B}}\right]\binom{N-1}{\frac{N-1}{2}}$$
$$=\frac{(1-B^2)^{\frac{N}{2}}}{2^N}\left[\frac{\sqrt{(1+B)^2}+\sqrt{(1-B)^2}}{\sqrt{1-B^2}}\right]\binom{N-1}{\frac{N-1}{2}}=\frac{(1-B^2)^{\frac{N}{2}-\frac{1}{2}}}{2^N}\left(1+B+1-B\right)\binom{N-1}{\frac{N-1}{2}}=\frac{(1-B^2)^{\frac{N}{2}-\frac{1}{2}}}{2^{N-1}}\binom{N-1}{\frac{N-1}{2}}. \tag{S27}$$

Simplifying the remaining terms in the first line of Eq. S26 yields

$$\frac{B(1+B)^{N-1}}{2^{N-1}}\left[\left(\frac{2}{1+B}\right)^{N-1}-\left(\frac{1-B}{1+B}\right)^{\frac{N-1}{2}}\binom{N-1}{\frac{N-1}{2}}\right]=B-\frac{B(1+B)^{N-1}}{2^{N-1}}\left(\frac{1-B}{1+B}\right)^{\frac{N-1}{2}}\binom{N-1}{\frac{N-1}{2}}$$
$$=B-\frac{B(1+B)^{\frac{N}{2}-\frac{1}{2}}}{2^{N-1}}\left(1-B\right)^{\frac{N}{2}-\frac{1}{2}}\binom{N-1}{\frac{N-1}{2}}=B-\frac{B(1-B^2)^{\frac{N}{2}-\frac{1}{2}}}{2^{N-1}}\binom{N-1}{\frac{N-1}{2}}. \tag{S28}$$

The sum of Eqs. S27 and S28 is given by

$$\frac{(1-B^2)^{\frac{N}{2}-\frac{1}{2}}}{2^{N-1}}\binom{N-1}{\frac{N-1}{2}}+B-\frac{B(1-B^2)^{\frac{N}{2}-\frac{1}{2}}}{2^{N-1}}\binom{N-1}{\frac{N-1}{2}}=B+\frac{(1-B^2)^{\frac{N}{2}-\frac{1}{2}}}{2^{N-1}}\binom{N-1}{\frac{N-1}{2}}\left(1-B\right)=B+(1-B)\frac{(1-B^2)^{\frac{N}{2}-\frac{1}{2}}}{2^{N-1}}\binom{2m}{m} \tag{S29}$$

where in the last step we used $m$ as defined in Eq. S16. The term containing the hypergeometric function in Eq. S26 simplifies as follows:

$$\frac{B(1+B)^{N-1}}{2^{N-1}}\left[-2\frac{(2m)!}{(m+1)!(m-1)!}\left(\frac{1-B}{1+B}\right)^{m+1}{}_2F_1\left(1;\frac{3}{2}-\frac{N}{2};\frac{N}{2}+\frac{3}{2};\frac{B-1}{B+1}\right)\right]. \tag{S30}$$

The prefactor of the hypergeometric function in S30 can be further reduced to:

$$-2\binom{2m}{m+1}\left(\frac{1-B}{1+B}\right)^{m+1}\frac{B(1+B)^{2m}}{2^{N-1}}=-\frac{B(1-B)^{m+1}(1+B)^{m-1}}{2^{N-2}}\binom{2m}{m+1}=-\frac{B(1-B)^{m+1}(1+B)^{m-1}}{2^{N-2}}\frac{m}{m+1}\binom{2m}{m}$$
$$=-\frac{B(1-B)^{\frac{N}{2}+\frac{1}{2}}(1+B)^{\frac{N}{2}-\frac{3}{2}}}{2^{N-2}}\frac{\frac{N-1}{2}}{\frac{N+1}{2}}\binom{N-1}{\frac{N-1}{2}}=-\frac{B(1-B)^{\frac{1}{2}}(1-B^2)^{\frac{N}{2}}}{2^{N-2}(1+B)^{\frac{3}{2}}}\frac{N-1}{N+1}\binom{N-1}{\frac{N-1}{2}}. \tag{S31}$$

Summing all terms appearing in Eq. S26 yields

$$S_{\text{odd}}(N,B)=B+\frac{(1-B^2)^{\frac{N}{2}}}{2^{N-2}}\binom{N-1}{\frac{N-1}{2}}\left[\frac{1}{2}\sqrt{\frac{1-B}{1+B}}-\frac{B(1-B)^{\frac{1}{2}}}{(1+B)^{\frac{3}{2}}}\frac{N-1}{N+1}{}_2F_1\left(1;\frac{3}{2}-\frac{N}{2};\frac{N}{2}+\frac{3}{2};\frac{B-1}{B+1}\right)\right]$$
$$=B+\frac{(1-B^2)^{\frac{N}{2}}}{2^{N-1}}\binom{N-1}{\frac{N-1}{2}}\sqrt{\frac{1-B}{1+B}}\left[1-\frac{2B}{1+B}\frac{N-1}{N+1}{}_2F_1\left(1;\frac{3}{2}-\frac{N}{2};\frac{N}{2}+\frac{3}{2};\frac{B-1}{B+1}\right)\right]. \tag{S32}$$

This result can also be written in terms of $p$ and $q$ as

$$S_{\text{odd}}(N,p,q)=(p-q)+2(pq)^{\frac{N}{2}}\sqrt{\frac{q}{p}}\binom{N-1}{\frac{N-1}{2}}\left[1+\frac{N-1}{N+1}\left(\frac{q}{p}-1\right){}_2F_1\left(1;\frac{3}{2}-\frac{N}{2};\frac{N}{2}+\frac{3}{2};-\frac{q}{p}\right)\right]. \tag{S33}$$

## Obtaining the survival probability in closed-form for even step numbers (Eq. 4b of main text)

In the case of even step numbers $N$, let us define $N = 2m$. We can thus simplify the floor functions

$$\left\lfloor \frac{N-1}{2} \right\rfloor = m - 1 \qquad N - \left\lfloor \frac{N-1}{2} \right\rfloor = (2m) - (m-1) = m + 1 \tag{S34}$$

appearing in the summation term of Eq. S12, which was defined as $\tilde{S}(N,B)$ in Eq. S13. Rewriting $\tilde{S}(N,B)$ in terms of $y = N - 1 - x$ as in Eq. S15 yields

$$\begin{aligned}\tilde{S}(N,B) &= \frac{B(1+B)^{N-1}}{2^{N-1}}\left[(1+\beta)^{N-1} - \sum_{x=m-1}^{N-1} \beta^x \binom{N-1}{x} - \sum_{y=m+1}^{N-1} \beta^y \binom{N-1}{y}\right] \\ &= \frac{B(1+B)^{N-1}}{2^{N-1}}\left[(1+\beta)^{N-1} - \beta^{m-1}\binom{2m-1}{m-1} - \beta^m \binom{2m-1}{m} - 2\sum_{y=m+1}^{2m-1} \beta^y \binom{2m-1}{y}\right].\end{aligned} \tag{S35}$$

where $\beta = \frac{1-B}{1+B}$. The remaining summation

$$\sum_{y=m+1}^{2m-1} \beta^y \binom{2m-1}{y} = \sum_{y=m+1}^{2m-1} \beta^y \frac{(2m-1)!}{y!(2m-y-1)!} \tag{S36}$$

can be expressed in terms of a hypergeometric function. To see this, note that $(m-2)! = (m-2)(m-3)...(2m-y)(2m-y-1)!$. Therefore the summation of Eq. S36 becomes

$$\begin{aligned}\sum_{y=m+1}^{2m-1} \frac{(2m-1)!}{y!}\beta^y \frac{(2m-y)...(m-3)(m-2)}{(m-2)!} &= \sum_{y=m+1}^{2m-1} \left[\frac{(2m-y)...(m-3)(m-2)}{y(y-1)...(m+3)(m+2)(m+1)!}\beta^{y-m-1}\beta^{m+1}\frac{(2m-1)!}{(m-2)!}\right] \\ &= \frac{\beta^{m+1}(2m-1)!}{(m+1)!(m-2)!}\sum_{y=m+1}^{2m-1}\left[\frac{(2m-y)...(m-3)(m-2)}{y(y-1)...(m+3)(m+2)}\beta^{y-m-1}\right].\end{aligned} \tag{S37}$$

Letting $n = y - m - 1$, the summation of Eq. S36 becomes the following:

$$\sum_{y=m+1}^{2m-1} \beta^y \binom{2m-1}{y} = \frac{\beta^{m+1}(2m-1)!}{(m+1)!(m-2)!}\sum_{n=0}^{m-2} \frac{(m-n-1)...(m-3)(m-2)}{(m+n+1)(m+n)...(m+3)(m+2)}\beta^n . \tag{S38}$$

Similar to the method employed for odd $N$ in the previous section, we multiply and divide the summand by $n!$, and also multiply the summand by $(-1)^{2n}$:

$$\sum_{y=m+1}^{2m-1} \beta^y \binom{2m-1}{y} = \frac{\beta^{m+1}(2m-1)!}{(m+1)!(m-2)!}\sum_{n=0}^{m-2} \frac{(m-n-1)...(m-3)(m-2)(-1)^{2n}}{(m+n+1)(m+n)...(m+3)(m+2)}\frac{n!}{n!}\beta^n . \tag{S39}$$

We now pair a factor $(-1)^n$ with $\beta^n$, and pair the other $(-1)^n$ factor with $(m-n-1)...(m-3)(m-2)$ to give $(2-m)(3-m)...(2-m+n-1)$. Using the falling Pochhammer symbol $(r)_n$ as defined in Eq. S23, we obtain

$$\sum_{y=m+1}^{2m-1} \beta^y \binom{2m-1}{y} = \frac{\beta^{m+1}(2m-1)!}{(m+1)!(m-2)!}\sum_{n=0}^{m-2} \frac{(1)_n(2-m)_n}{(m+2)_n}\frac{(-\beta)^n}{n!} \tag{S40}$$

and noting that $(2-m)_n = 0$ for all $n > m-2$, we arrive at an expression in terms of the hypergeometric function:

$$\sum_{y=m+1}^{2m-1} \beta^y \binom{2m-1}{y} = \frac{\beta^{m+1}(2m-1)!}{(m+1)!(m-2)!}\sum_{n=0}^{\infty} \frac{(1)_n(2-m)_n}{(m+2)_n}\frac{(-\beta)^n}{n!} = \frac{\beta^{m+1}(2m-1)!}{(m+1)!(m-2)!}\,{}_2F_1(1; 2-m; m+2; -\beta)\,. \tag{S41}$$

Therefore, the survival probability of Eq. S12 becomes

$$\begin{aligned}S_{\text{even}} =& \left[\frac{(1+B)^{\lceil\frac{N+1}{2}\rceil}(1-B)^{\lfloor\frac{N-1}{2}\rfloor} + (1+B)^{\lfloor\frac{N-1}{2}\rfloor}(1-B)^{\lceil\frac{N+1}{2}\rceil}}{2^N}\right]\binom{N-1}{\lfloor\frac{N-1}{2}\rfloor} + \frac{B(1+B)^{N-1}}{2^{N-1}}\left[\left(\frac{2}{1+B}\right)^{N-1} - \left(\frac{1-B}{1+B}\right)^{\lfloor\frac{N-1}{2}\rfloor}\binom{N-1}{\lfloor\frac{N-1}{2}\rfloor}\right. \\ &\left. - \left(\frac{1-B}{1+B}\right)^{\lfloor\frac{N}{2}\rfloor}\binom{N-1}{\lfloor\frac{N}{2}\rfloor} - \frac{2(N-1)!}{(\lfloor\frac{N+2}{2}\rfloor)!(\lfloor\frac{N-3}{2}\rfloor)!}\left(\frac{1-B}{1+B}\right)^{\lfloor\frac{N+2}{2}\rfloor} {}_2F_1\left(1; 1-\left\lfloor\frac{N-1}{2}\right\rfloor; \left\lfloor\frac{N+4}{2}\right\rfloor; \frac{B-1}{B+1}\right)\right].\end{aligned} \tag{S42}$$

The factorials in the hypergeometric function's prefactor can be simplified as follows by virtue of $N$ being even:

$$\frac{(N-1)!}{(\lfloor\frac{N+2}{2}\rfloor)!(\lfloor\frac{N-3}{2}\rfloor)!} = \frac{(N-1)!}{(\frac{N}{2}+1)!(\frac{N}{2}-2)!} = \binom{N-1}{\frac{N}{2}+1}. \tag{S43}$$

Let us now examine the two terms preceding the hypergeometric term in Eq. S42:

$$-\left(\frac{1-B}{1+B}\right)^{\frac{N}{2}-1}\binom{N-1}{\frac{N}{2}-1} - \left(\frac{1-B}{1+B}\right)^{\frac{N}{2}}\binom{N-1}{\frac{N}{2}}. \tag{S44}$$

Using the binomial identity

$$\binom{n}{x} = \binom{n-1}{x-1} + \binom{n-1}{x} \quad\longrightarrow\quad \binom{N-1}{\frac{N}{2}} = \binom{N}{\frac{N}{2}} - \binom{N-1}{\frac{N}{2}-1} \tag{S45}$$

we rewrite Eq. S44 as

$$-\left(\frac{1-B}{1+B}\right)^{\frac{N}{2}-1}\binom{N-1}{\frac{N}{2}-1} - \left(\frac{1-B}{1+B}\right)^{\frac{N}{2}}\binom{N-1}{\frac{N}{2}} = \left[1-\left(\frac{1-B}{1+B}\right)^{-1}\right]\left(\frac{1-B}{1+B}\right)^{\frac{N}{2}}\binom{N-1}{\frac{N}{2}-1} - \left(\frac{1-B}{1+B}\right)^{\frac{N}{2}}\binom{N}{\frac{N}{2}}. \tag{S46}$$

Thus $S_{\text{even}}(N,B)$ becomes

$$\begin{aligned} S_{\text{even}} = &\left[\frac{(1+B)^{\frac{N}{2}+1}(1-B)^{\frac{N}{2}-1} + (1+B)^{\frac{N}{2}-1}(1-B)^{\frac{N}{2}+1}}{2^N}\right]\binom{N-1}{\frac{N}{2}-1} + \frac{B(1+B)^{N-1}}{2^{N-1}}\left[\left(\frac{2}{1+B}\right)^{N-1} - \left(\frac{1-B}{1+B}\right)^{\frac{N}{2}}\binom{N}{\frac{N}{2}}\right. \\ &\left. + \left\{1-\left(\frac{1+B}{1-B}\right)\right\}\left(\frac{1-B}{1+B}\right)^{\frac{N}{2}}\binom{N-1}{\frac{N}{2}-1} - 2\binom{N-1}{\frac{N}{2}+1}\left(\frac{1-B}{1+B}\right)^{\frac{N}{2}+1} {}_2F_1\left(1;2-\frac{N}{2};\frac{N}{2}+2;\frac{B-1}{B+1}\right)\right]. \end{aligned} \tag{S47}$$

Further simplifying,

$$\begin{aligned} S_{\text{even}} = &\left[\frac{(1+B)^{\frac{N}{2}+1}(1-B)^{\frac{N}{2}-1} + (1+B)^{\frac{N}{2}-1}(1-B)^{\frac{N}{2}+1}}{2^N}\right]\binom{N-1}{\frac{N}{2}-1} + B - \frac{B(1+B)^{N-1}}{2^{N-1}}\left(\frac{1-B}{1+B}\right)^{\frac{N}{2}}\binom{N}{\frac{N}{2}} \\ &+ \frac{B(1+B)^{N-1}}{2^{N-1}}\left[1-\left(\frac{1+B}{1-B}\right)\right]\left(\frac{1-B}{1+B}\right)^{\frac{N}{2}}\binom{N-1}{\frac{N}{2}-1} - \frac{B(1+B)^{N-1}}{2^{N-2}}\binom{N-1}{\frac{N}{2}+1}\left(\frac{1-B}{1+B}\right)^{\frac{N}{2}+1} {}_2F_1\left(1;\frac{4-N}{2};\frac{N+4}{2};\frac{B-1}{B+1}\right) \\ = &\ B + \left[\frac{(1+B)^{\frac{N}{2}+1}(1-B)^{\frac{N}{2}-1} + (1+B)^{\frac{N}{2}-1}(1-B)^{\frac{N}{2}+1}}{2^N}\right]\binom{N-1}{\frac{N}{2}-1} - \frac{B(1+B)^{\frac{N}{2}-1}(1-B)^{\frac{N}{2}}}{2^{N-1}}\binom{N}{\frac{N}{2}} \\ &+ \left[\frac{B(1+B)^{\frac{N}{2}-1}(1-B)^{\frac{N}{2}}}{2^{N-1}} - \frac{B(1+B)^{\frac{N}{2}}(1-B)^{\frac{N}{2}-1}}{2^{N-1}}\right]\binom{N-1}{\frac{N}{2}-1} - \frac{B(1+B)^{\frac{N}{2}-2}(1-B)^{\frac{N}{2}+1}}{2^{N-2}}\binom{N-1}{\frac{N}{2}+1} {}_2F_1\left(1;2-\frac{N}{2};\frac{N}{2}+2;\frac{B-1}{B+1}\right) \end{aligned} \tag{S48}$$

Combining terms with the binomial coefficient $\binom{N-1}{\frac{N}{2}-1}$, and factoring out $(1+B)^{\frac{N}{2}}(1-B)^{\frac{N}{2}} = (1-B^2)^{\frac{N}{2}}$ yields:

$$S_{\text{even}} = B + \frac{(1-B^2)^{\frac{N}{2}}}{2^{N-1}}\binom{N-1}{\frac{N}{2}-1} - \frac{B(1-B^2)^{\frac{N}{2}}}{2^{N-1}(1+B)}\binom{N}{\frac{N}{2}} - \frac{B(1-B^2)^{\frac{N}{2}}(1-B)}{2^{N-2}(1+B)^2}\binom{N-1}{\frac{N}{2}+1} {}_2F_1\left(1;2-\frac{N}{2};\frac{N}{2}+2;\frac{B-1}{B+1}\right) \tag{S49}$$

Next we note that the binomial coefficient

$$\binom{N-1}{\frac{N}{2}+1} = \frac{N-2}{N+2}\binom{N-1}{\frac{N}{2}-1} = \frac{1}{2}\frac{N-2}{N+2}\binom{N}{\frac{N}{2}} \tag{S50}$$

where the following binomial identity was used in the last equality:

$$\binom{n-1}{x-1} = \frac{x}{n}\binom{n}{x}. \tag{S51}$$

The survival probability thus simplifies as:

$$S_{\text{even}}(N,B) = B + \frac{(1-B^2)^{\frac{N}{2}}}{2^N}\binom{N}{\frac{N}{2}} - \frac{B(1-B^2)^{\frac{N}{2}}}{2^{N-1}(1+B)}\binom{N}{\frac{N}{2}} - \frac{B(1-B^2)^{\frac{N}{2}}(1-B)}{2^{N-1}(1+B)^2}\frac{N-2}{N+2}\binom{N}{\frac{N}{2}} {}_2F_1\left(1;2-\frac{N}{2};\frac{N}{2}+2;\frac{B-1}{B+1}\right) \tag{S52}$$

and we arrive at the final result (Eq. 4b of the main text):

$$S_{\text{even}}(N,B) = B + \frac{(1-B^2)^{\frac{N}{2}}}{2^N}\binom{N}{\frac{N}{2}}\left[1 - \frac{2B}{1+B} - 2B\frac{1-B}{(1+B)^2}\frac{N-2}{N+2}\,{}_2F_1\!\left(1;2-\frac{N}{2};2+\frac{N}{2};\frac{B-1}{B+1}\right)\right]$$
$$= B + \frac{(1-B^2)^{\frac{N}{2}}}{2^N}\binom{N}{\frac{N}{2}}\left[\frac{1-B}{1+B} - 2B\frac{1-B}{(1+B)^2}\frac{N-2}{N+2}\,{}_2F_1\!\left(1;2-\frac{N}{2};2+\frac{N}{2};\frac{B-1}{B+1}\right)\right]. \quad \text{(S53)}$$

In terms of $p$ and $q$, this result can be written as:

$$S_{\text{even}}(N,p,q) = (p-q) + (pq)^{\frac{N}{2}}\binom{N}{\frac{N}{2}}\left[\frac{q}{p} + \frac{N-2}{N+2}\left[\left(\frac{q}{p}\right)^2 - \frac{q}{p}\right]{}_2F_1\!\left(1;2-\frac{N}{2};2+\frac{N}{2};-\frac{q}{p}\right)\right]. \quad \text{(S54)}$$

## Explicit formulae for $dS/dB$

Below are the explicit formulae for $dS/dB$ for even and odd step numbers, as plotted in Fig. 3 of the main text.

$$\frac{dS_{\text{even}}}{dB} = 1 + \frac{(1-B^2)^{N/2}}{2^N(1+B)^3}\binom{N}{\frac{N}{2}}\Bigg[-(1+B)(2+NB) + (2NB^2+6B-2)\frac{N-2}{N+2}\,{}_2F_1\left(1;2-\frac{N}{2};2+\frac{N}{2};\frac{B-1}{B+1}\right)$$
$$+ 4B\left(\frac{1-B}{1+B}\right)\left(\frac{N-4}{N+4}\right)\left(\frac{N-2}{N+2}\right){}_2F_1\left(2;3-\frac{N}{2};3+\frac{N}{2};\frac{B-1}{B+1}\right)\Bigg] \quad \text{(S55)}$$

$$\frac{dS_{\text{odd}}}{dB} = 1 + \frac{(1-B^2)^{N/2}}{2^N}\binom{N-1}{\frac{N-1}{2}}\sqrt{\frac{1-B}{1+B}}\Bigg\{-\frac{2(1+NB)}{1-B^2} + 4\left(\frac{N-1}{N+1}\right)\frac{NB^2+2B-1}{(1-B)(1+B)^2}\,{}_2F_1\left(1;\frac{3}{2}-\frac{N}{2};\frac{3}{2}+\frac{N}{2};\frac{B-1}{B+1}\right)$$
$$+ \frac{8B}{(1+B)^3}\left(\frac{N-3}{N+3}\right)\left(\frac{N-1}{N+1}\right){}_2F_1\left(2;\frac{5}{2}-\frac{N}{2};\frac{5}{2}+\frac{N}{2};\frac{B-1}{B+1}\right)\Bigg\} \quad \text{(S56)}$$

## Obtaining an expression for the first return time distribution from the survival probability

Recall from Eq. 7 of the main text that the probability of first return occurring at step $i$ is

$$F(i+1) = -(S(i+1) - S(i)). \quad \text{(S57)}$$

Because first return can only occur at even step numbers ($F$ is zero for odd step numbers), we define here $F(N)$ for even step numbers $N$ as:

$$F(N) = S_{\text{odd}}(N-1,B) - S_{\text{even}}(N,B)\,. \quad \text{(S58)}$$

Using the closed-form expressions Eqs. S32 and S53 for $S_{\text{odd}}$ and $S_{\text{even}}$, Eq. S58 becomes

$$F(N) = B + \frac{(1-B^2)^{\frac{N-1}{2}}}{2^{N-2}}\binom{N-2}{\frac{N-2}{2}}\sqrt{\frac{1-B}{1+B}}\left[1 - \frac{2B}{1+B}\frac{N-2}{N}\,{}_2F_1\!\left(1;-\frac{N-1}{2}+\frac{3}{2};\frac{N-1}{2}+\frac{3}{2};\frac{B-1}{B+1}\right)\right]$$
$$- B - \frac{(1-B^2)^{\frac{N}{2}}}{2^N}\binom{N}{\frac{N}{2}}\left[\frac{1-B}{1+B} - 2B\frac{1-B}{(1+B)^2}\frac{N-2}{N+2}\,{}_2F_1\!\left(1;-\frac{N}{2}+2;\frac{N}{2}+2;\frac{B-1}{B+1}\right)\right]$$
$$= \frac{(1-B^2)^{\frac{N}{2}}}{2^N}\binom{N-2}{\frac{N}{2}-1}\frac{1}{4(1+B)}\left[1 - \frac{2B}{1+B}\frac{N-2}{N}\,{}_2F_1\!\left(1;2-\frac{N}{2};\frac{N}{2}+1;\frac{B-1}{B+1}\right)\right]$$
$$- \frac{(1-B^2)^{\frac{N}{2}}}{2^N}\binom{N}{\frac{N}{2}}\left[\frac{1-B}{1+B} - 2B\frac{1-B}{(1+B)^2}\frac{N-2}{N+2}\,{}_2F_1\!\left(1;-\frac{N}{2}+2;\frac{N}{2}+2;\frac{B-1}{B+1}\right)\right]. \quad \text{(S59)}$$

Noting that

$$\binom{N-2}{\frac{N}{2}-1} = \frac{N}{4(N-1)}\binom{N}{\frac{N}{2}}, \quad \text{(S60)}$$

we obtain

$$
\begin{aligned}
F(N) =& \frac{(1-B^2)^{\frac{N}{2}}}{2^N}\binom{N-2}{\frac{N}{2}-1}\Big[\frac{1}{4(1+B)} - \frac{B}{2(1+B)^2}\,\frac{N-2}{N}\,{}_2F_1\Big(1;2-\frac{N}{2};\frac{N}{2}+1;\frac{B-1}{B+1}\Big)\Big] \\
&- \frac{(1-B^2)^{\frac{N}{2}}}{2^N}\binom{N}{\frac{N}{2}}\Big[\frac{1-B}{1+B} - 2B\,\frac{1-B}{(1+B)^2}\,\frac{N-2}{N+2}\,{}_2F_1\Big(1;-\frac{N}{2}+2;\frac{N}{2}+2;\frac{B-1}{B+1}\Big)\Big] \\
=& \frac{(1-B^2)^{\frac{N}{2}}}{2^N}\binom{N}{\frac{N}{2}}\Big[\frac{N}{16(1+B)(N-1)} - \frac{B}{8(1+B)^2}\,\frac{N-2}{N-1}\,{}_2F_1\Big(1;2-\frac{N}{2};\frac{N}{2}+1;\frac{B-1}{B+1}\Big)\Big] \\
&+ \frac{(1-B^2)^{\frac{N}{2}}}{2^N}\binom{N}{\frac{N}{2}}\Big[\frac{B-1}{B+1} + 2B\,\frac{1-B}{(1+B)^2}\,\frac{N-2}{N+2}\,{}_2F_1\Big(1;-\frac{N}{2}+2;\frac{N}{2}+2;\frac{B-1}{B+1}\Big)\Big]. \qquad \text{(S61)}
\end{aligned}
$$

Combining terms, the first return time distribution for even $N$ becomes:

$$
\begin{aligned}
F(N) =& \frac{(1-B^2)^{\frac{N}{2}}}{2^N}\binom{N}{\frac{N}{2}}\Big[\frac{N}{16(1+B)(N-1)} + \frac{B-1}{B+1} + 2B\,\frac{1-B}{(1+B)^2}\,\frac{N-2}{N+2}\,{}_2F_1\Big(1;2-\frac{N}{2};\frac{N}{2}+2;\frac{B-1}{B+1}\Big) \\
&- \frac{B}{8(1+B)^2}\,\frac{N-2}{N-1}\,{}_2F_1\Big(1;2-\frac{N}{2};\frac{N}{2}+1;\frac{B-1}{B+1}\Big)\Big]. \qquad \text{(S62)}
\end{aligned}
$$

## Obtaining the critical bias criterion (Eq. 10 of main text)

A PLR which decreases monotonically throughout a walk requires that $\mathrm{PLR}(1,B) < \mathrm{PLR}(1-1/n,B)$, where $\mathrm{PLR}(1,B) = \left(\frac{1-B^2}{4}\right)^n\binom{2n}{n}$ and

$$
\mathrm{PLR}(1-1/n,B) = \left(\frac{1-B^2}{4}\right)^{n(1-\frac{1}{n})}\binom{2n(1-\frac{1}{n})}{n(1-\frac{1}{n})}S_{\mathrm{even}}(2n(1-1+\frac{1}{n}),B) = \left(\frac{1-B^2}{4}\right)^{n-1}\binom{2n-2}{n-1}S_{\mathrm{even}}(2,B)\,. \qquad \text{(S63)}
$$

Thus our criterion becomes:

$$
\left(\frac{1-B^2}{4}\right)^n\binom{2n}{n} < \left(\frac{1-B^2}{4}\right)^{n-1}\binom{2n-2}{n-1}S_{\mathrm{even}}(2,B) \quad\longrightarrow\quad \binom{2n}{n} < \frac{4}{1-B^2}\binom{2n-2}{n-1}S_{\mathrm{even}}(2,B) \qquad \text{(S64)}
$$

which further simplifies to

$$
\frac{\binom{2n}{n}}{\binom{2n-2}{n-1}} = 4 - \frac{2}{n} < \left(\frac{4}{1-B^2}\right)S_{\mathrm{even}}(2,B) \quad\longrightarrow\quad (1-B^2)\left(1-\frac{1}{2n}\right) < S_{\mathrm{even}}(2,B)\,. \qquad \text{(S65)}
$$

Noting that

$$
S_{\mathrm{even}}(2,B) = B + \frac{1-B^2}{2}\left(1-\frac{2B}{1+B}\right) = B + \frac{1-B^2}{2} - \frac{(1-B)(1+B)}{2}\,\frac{2B}{1+B} = \frac{1+B^2}{2}\,, \qquad \text{(S66)}
$$

the critical bias criterion becomes

$$
(1-B^2)\left(1-\frac{1}{2n}\right) < \frac{1+B^2}{2} \quad\longrightarrow\quad 1-\frac{1}{n} < B^2\left(3-\frac{1}{n}\right) \quad\longrightarrow\quad \frac{n-1}{3n-1} < B^2\,. \qquad \text{(S67)}
$$

We thus obtain the condition given in Eq. 10 of the main text:

$$
|B| > \sqrt{\frac{n-1}{3n-1}}\,. \qquad \text{(S68)}
$$

# References


[1] M. Renault, Four proofs of the ballot theorem, Mathematics magazine, **80**(5), 345-352 (2007).

[2] M. Abramowitz and I. A. Stegun, *Handbook of Mathematical Functions with Formulas, Graphs, and Mathematical Tables* (Dover, New York, 1942) 9th ed.
